# Supplementary material for: MASKDROID: Robust Android Malware Detection with Masked Graph Representations
Source: arXiv:2409.19594 source file (2024-09-29)
Supplement: Supplementary file 1 [file 8_appendix.tex]

\appendix
\clearpage
\section{Experimental Settings}  \label{sec:app_set}
\subsection{Datasets.} \label{sec:app_datasets}

\subsection{Baselines} \label{sec:app_baselines}

\subsection{Parameter Settings and Training Cost}

\subsection{Additional Experiments} \label{sec:app_3d}
